# Supplementary material for: Learning to Recorrupt: Noise Distribution Agnostic Self-Supervised Image Denoising
Source: arXiv:2603.25869 source file (2026-09-28)
Supplement: Supplementary file 1 [file supplementary.tex]

\documentclass{article}

% Import additional packages in the preamble file, before hyperref
\input{preamble}
\usepackage{xcolor,colortbl}
\usepackage{graphicx}
\usepackage{amsmath}
\usepackage{amssymb}
\usepackage{booktabs}
\usepackage{amsthm}
\usepackage{comment}
\usepackage{cancel}
\usepackage[margin=.8in]{geometry}
\usepackage{hyperref}
\usepackage{wrapfig}

\begin{document}

\input{sec/X_suppl}

\;\;

\break
{
    \small
    \bibliographystyle{IEEEtran}
    \bibliography{main}
}

\end{document}
